# Supplementary material for: Towards Generalizable Multi-Camera 3D Object Detection via Perspective Debiasing
Source: arXiv:2310.11346 source file (2023-12-25)
Supplement: Supplementary file 1 [file appendix.tex]

\section{Additional Details for Theoretical Analysis}\label{app:theory}
\subsection{Derivation and Analysis of Image A to Image B Projection}\label{app:theory_proj}
In this section, we derive our formulation for the projection $(x_b, y_b, d_b)$ in Equation \ref{eq:proj} and connect it to the familiar standard stereo case. 

Starting from Image A coordinates $(x_a, y_a, d_a)$ and applying homographic transforms:
\begin{align}
    [x_a, y_a, d_a] &\implies [x_a d_a, y_a d_a, d_a] \tag{Image A Image Hom Coords} \\
    &\implies \left[ \frac{d_a (x_a - c_x)}{f}, \frac{d_a (y_a - c_y)}{f}, d_a \right] \tag{Image A Camera Coords} \\
    &\implies \left[ \frac{d_a x_a'}{f}, \frac{d_a y_a'}{f}, d_a \right] \tag{Let $x_a' = x_a - c_x, y_a' = y_a - c_y$} \\
    &\implies \left[ 
        \frac{d_a x_a' \cos{\theta}}{f} - d_a \sin{\theta} + t_x,
        \frac{d_a y_a'}{f},
        \frac{d_a x_a' \sin{\theta}}{f} + d_a \cos{\theta} + t_z
    \right] \tag{Image B Camera Coords} \\
    &\implies \begin{aligned}\Bigg[&
        \frac{d_a x_a' \cos{\theta} - d_a f \sin{\theta} + t_x f}{\frac{d_a x_a' \sin{\theta}}{f} + d_a \cos{\theta} + t_z} + c_x, \\
        &~~~~~\frac{d_a y_a'}{\frac{d_a x_a' \sin{\theta}}{f} + d_a \cos{\theta} + t_z} + c_y, \\
        &~~~~~\frac{d_a x_a' \sin{\theta}}{f} + d_a \cos{\theta} + t_z
    \Bigg]\end{aligned} \tag{Image B Image Coords} \\
    &~~= [x_b, y_b, d_b] \tag{Image B Image Coords}
\end{align}

This formulation is applicable to any two-camera system with rotation and translation along the XZ axis. For instance, consider a standard stereo setup with cameras $A$ and $B$ as the left and right cameras, respectively: $\theta = 0$, $t_z = 0$, baseline $-t_x > 0$. Then, the above reduces to:
\[
[x_b, y_b, d_b] = \left[\frac{d_a x_a' + t_x f}{d_a} + c_x, \frac{d_a y_a'}{d_a} + c_y, d_a\right] = \left[x_a - \frac{t_x f}{d_a}, y_a, d_a \right]
\]
This yields the standard stereo disparity formula $disparity = \frac{t_x f}{d_a}$. For depth estimation in stereo or temporal stereo, we project multiple depth hypotheses for a pixel in image A onto image B and find the pixel along the epipolar line in image B that matches best with the original pixel in image A. Given such a matching, we can derive the depth using the transformation matrix between the two images/cameras. For such a formulation to work well, it is beneficial for the image B projections of nearby depth hypotheses for a pixel in image A to be as far apart from one another as possible. For instance, if two candidate depths are projected to the same pixel in image B, it is impossible to determine which of the two candidates are a better match. Even beyond same-pixel projections, with downsampled feature maps and local homogeneity of features extracted from CNN backbones, more separated depth hypothesis projections allows for easier stereo depth estimation. To quantify changes in projection from changes in depth, we defined in the main paper localization potential, which is closely tied to the ease of depth estimation.

We then examine localization potential in this standard stereo case by finding $\lvert \frac{\partial x_b}{\partial d_a} \rvert$. For the standard stereo setup, $\lvert \frac{\partial x_b}{\partial d_a} \rvert = \frac{(-t_x) f}{d_a^2}$. This partial derivative tells us that localization potential is larger, which means depth estimation is easier, if:
\begin{itemize}
    \item The baseline $-t_x$ is larger. This is in-line with our intuition; the further apart the cameras are, smaller depth changes can be captured. 
    \item The focal length $f$ is larger. Intuitively, if we downsample the image resolution, the focal length decreases, causing more different depth hypotheses to project to the now ''larger'' pixels.
    \item The depth at which we evaluate localization potential is smaller. Indeed, the projected difference between 1m and 2m is larger than the difference between 59m and 60m.
\end{itemize}

We do comment, however, that these observations do not mean the depth estimation quality in standard stereo can be simply improved by adopting a larger baseline and focal length. A larger baseline significantly decreases the overlapping region in standard stereo while a larger focal length limits the scene captured. In addition, we observe that unlike the general two-view case in Equation \ref{eq:math_localization_potential}, the localization potential does not vary over different image A x-coordinates for standard stereo. This is because the stereo cameras are aligned, causing the epipolar lines to be parallel to the x axis. As such, choosing an optimal setup for standard stereo is much simpler compared to the more general multi-view, temporal stereo case.

\subsection{Full Proof of Formulation of Localization Potential}\label{app:theory_loc_potential}
In this section, we detail the steps we took to derive our formulation for localization potential in Equation \ref{eq:math_localization_potential}. We first reparameterize $x_b$ using $\alpha$ as defined in Figure \ref{fig:coords}. Let $r_a' = \sqrt{(x_a')^2 + f^2}$ and note that we have $\sin{\alpha} = \frac{x_a'}{r_a'}, \cos{\alpha} = \frac{f}{r_a'}$. 
\begin{align*}
x_b &= \frac{d_a x_a' \cos{\theta} - d_a f \sin{\theta} + t_x f}{\frac{d_a x_a' \sin{\theta}}{f} + d_a \cos{\theta} + t_z} + c_x \\
    &= f \frac{d_a x_a' \cos{\theta} - d_a f \sin{\theta} + t_x f}{d_a x_a' \sin{\theta} + d_a f \cos{\theta} + t_z f} + c_x \tag{multiply top \& bottom with $f$} \\
    &= f \frac{d_a r_a' \left(\frac{x_a'}{r_a'} \cos{\theta} - \frac{f}{r_a'} \sin{\theta}\right) + t_x f}{d_a r_a' \left( \frac{x_a'}{r_a'} \sin{\theta} + \frac{f}{r_a'} \cos{\theta} \right) + t_z f} + c_x \\
    &= f \frac{d_a r_a' \left(\sin{\alpha} \cos{\theta} - \cos{\alpha}  \sin{\theta}\right) + t_x f}{d_a r_a' \left( \sin{\alpha} \sin{\theta} + \cos{\alpha} \cos{\theta} \right) + t_z f} + c_x \tag{substitute $\sin{\alpha}, \cos{\alpha}$}\\
    &= f \frac{d_a r_a' \sin(\alpha - \theta) + t_x f}{d_a r_a' \cos(\alpha - \theta) + t_z f} + c_x \tag{sin \& cos identities} \\
    &= f \frac{d_a \sin(\alpha - \theta) + t_x \frac{f}{r_a'}}{d_a \cos(\alpha - \theta) + t_z \frac{f}{r_a'}} + c_x \tag{divide top \& bottom with $r_a'$} \\
    &= \frac{d_a f \sin(\alpha - \theta) + t_x f \cos{\alpha}}{d_a \cos(\alpha - \theta) + t_z \cos{\alpha}} + c_x \tag{substitute $\cos{\alpha}$} \\
\end{align*}
Then, deriving $\frac{\partial x_b}{\partial d_a}$ from this formulation, we get:
\[
\left\lvert \frac{\partial x_b}{\partial d_a} \right\rvert = \frac{f \cos(\alpha) |t_z \sin(\alpha - \theta) - t_x \cos(\alpha - \theta)|}{(d_a \cos(\alpha - \theta) + t_z\cos(\alpha))^2}
\]
Note that $\cos(\alpha) > 0$ for all values of $\alpha$. We can then rewrite the above further by using the angular direction of translation $\beta$ as defined in Figure \ref{fig:coords}. The total magnitude of translation is $\bar{t} = \sqrt{t_x^2 + t_y^2}$, giving us $\sin{\beta} = t_x/\bar{t}, \cos{\beta} = t_z/\bar{t}$. Then, we get:
\begin{align*}
    \left\lvert \frac{\partial x_b}{\partial d_a} \right\rvert &= \frac{f \cos(\alpha) |t_z \sin(\alpha - \theta) - t_x \cos(\alpha - \theta)|}{(d_a \cos(\alpha - \theta) + t_z\cos(\alpha))^2} \\
    &= \frac{f \bar{t} \cos(\alpha) |\cos(\beta) \sin(\alpha - \theta) - \sin(\beta) \cos(\alpha - \theta)|}{(d_a \cos(\alpha - \theta) + t_z\cos(\alpha))^2} \\
    &= \frac{f \bar{t} \cos(\alpha) |\sin(\alpha - (\theta + \beta))|}{(d_a \cos(\alpha - \theta) + t_z\cos(\alpha))^2}
\end{align*}
which is our formulation in Equation \ref{eq:math_localization_potential}.

\subsection{Effect of View Rotation $\theta$ on Localization Potential}\label{app:theory_rot}
In this section, we identify the impact of $\theta$ on localization potential formulation in Equation \ref{eq:math_localization_potential}. Again, recall that a larger value of $\left\lvert \frac{\partial x_b}{\partial d_a} \right\rvert$ means easier depth estimation. \textit{Critically}, we first observe that $\theta$ only affects the ease of depth estimation of a pixel through its \textit{relative} angular difference with $\alpha$ of that pixel and $\beta$. This is important because it means there is no singular camera rotation that is best for all pixels or all camera translations. The optimal rotation maximizing localization potential changes based on the pixel and the current ego-motion.

Analyzing Equation \ref{eq:math_localization_potential}, we find that if $\theta$ is close to $\alpha$, the $d_a\cos(\alpha - \theta)$ term increases, making the depth estimation more difficult by a factor of $d_a^2$. This is in-line with our intuition; if the camera rotation is such that the resulting camera B's principal axis is in-line with the pixel ray, the depth hypotheses along that pixel ray be projected close together. Further, we also want $\theta + \beta$ to be different from $\alpha$ (otherwise the numerator decreases). This follows a similar intuition as before - for depth hypotheses along a pixel ray to be projected further apart, the ego-vehicle should not rotate towards or move in the same direction as the pixel ray. 

\input{iclr2023/images_latex/optimal_theta}

We empirically verify our analysis by visualizing the optimal $\theta$ that maximizes localization potential over various depths and X-axis Image A Coordinates for the six cameras in nuScenes. For translational movement, we take the average ego-motion for moving scenes in nuScenes, which yields approximately $tx = 0.05m, tz = 3.19m$ between consecutive frames (0.5s difference) in the front camera coordinates. The results are shown in Figure \ref{fig:optimal_theta}. Indeed, we find that \textbf{the optimal $\theta$ various over different pixel locations, depths, and cameras}, varying most significantly over image location. As the translation direction $\beta$ is different for each camera, each with its own coordinate system, by observing varied rotation values over different cameras, we verify that translation direction significantly affects the optimal $\theta$ as well. Examining the front camera with translation direction $\beta$ close to 0, we find that the $\theta$ seeks to maximize the difference between $\alpha - \theta$ while keeping the candidate point in-view. Furthermore, the optimal $\theta$ does change over depth as well. For instance, the optimal $\theta$ along the center ray in the back right camera changes from 0 degrees at 10m to 30 degrees at 50m. That some \textbf{candidate locations prefer smaller rotations} runs contrary to methods used to choose matching frames in indoor temporal stereo, which impose a minimum rotation and translation \citep{Hou2019MultiViewSB,Sun2021NeuralReconRC} between frames to be used to for matching. Hence, there is no globally optimal rotation between views. \textbf{To allow different candidate locations to maximize their localization potential, it is important to utilize many views with different rotations irrespective of their magnitude.} In practice, we can obtain diverse rotations by utilizing many timesteps over long history.

\subsection{Optimal Time Difference Considering Multi-Camera Projection}\label{app:theory_optimal_time_cam}
We first further analyze trends in optimal time difference in \ref{fig:optimal_time}
Intuitively, for the forward-facing cameras where a larger time difference increases the distance between a 3D point and the vehicle, this is a trade-off between the tendency of further depth points to be projected closer together (the denominator) and the larger difference in views generated through ego-motion (the numerator). The former wins out for closer points and the latter for further points. The different trends over various cameras are representative of both their orientation w.r.t ego-vehicle movement (we see tilted trends for the left/right slanted cameras) as well as their general forward/backward facing orientation.
\input{iclr2023/images_latex/optimal_time_all_cams}
\input{iclr2023/images_latex/optimal_values_comparison}
Next, we visualize the optimal time difference for candidate locations when allowing for projections different cameras. We also visualize the optimal target camera that the depth hypothesis is projected onto. The results are in Figure \ref{fig:optimal_time_all_cams}. Further, we also maximized log localization potential values at these optimal locations in Figure \ref{fig:optimal_values_comparison}. First, we notice that in the multi-camera setup, all depth hypotheses have valid projections. This is important for two reasons. First, this allows all pixel locations and depths to benefit from multi-view depth estimation. Second, it allows the multi-camera setting to exploit larger temporal differences without worrying about non-overlapping regions. To see this, consider the back camera in Figure \ref{fig:optimal_values_comparison}. When considering multiple timesteps (row 1 to row 2), we see that the localization potential dramatically increases for regions where same-camera projections are valid. However, the close-depth regions are unable to make use of the larger temporal differences due to invalid same-camera projection. However, when considering all cameras, we are able to leverage larger temporal differences for both these close-depth and previously invalid regions. In standard stereo, a larger baseline, despite the easier depth estimation, causes large portions of the left \& right images to not overlap. However, via our formulation, in multi-timestep temporal stereo with multiple cameras, we can leverage larger temporal differences without worrying about lack of overlap. Finally, we also notice that the multi-camera setup, although better for localization potential, has much more complex patterns for optimal time difference compared to the single-camera setup. Similar to our conclusions when analyzing rotation, we find that the optimal time difference various for different pixels, cameras, ego-motion, depth, and camera setup.

\subsection{Optimal Time Difference during Ego-Vehicle Rotation}\label{app:theory_turns}
\input{iclr2023/images_latex/optimal_time_all_cams_rot}
In this section, we consider the case where theta varies with time. This happens during ego-vehicle turns, and we visualize the optimal time difference over the candidate locations in realistic scenarios of 30, 60, and 90 degree turns in Figure \ref{fig:optimal_time_all_cams_rot}. We find that when $\theta$ varies with time, the optimal time difference and optimal projected camera varies wildly over different candidate locations. This shows that it is suboptimal to choose just a few temporal differences for multi-view stereo - a past frame that worked well when the vehicle simply moved forward might fail drastically in more complex ego-motion scenarios such as turns. As such, we conclude it is not only optimal but also necessary to leverage many past timesteps over a long time window for multi-view stereo.

\subsection{Additional Analysis on Effects of Temporal Difference on Multi-View Depth Ambiguity}\label{app:theory_ambig}
\input{iclr2023/images_latex/boxplot_effective_disparities}
We find that with the single timestep aggregation used in many methods, less than 20 \% of change in object center projection is larger than 1 pixel for objects at 40m - 60m, making accurate multi-view localization impossible. By leveraging 16 past timesteps, we significantly ease multi-view depth estimation (note that for frames with less than 16 timesteps of history, we use as many is available). We do note, however, that the critical front camera is the most difficult view. This is because as seen in Figure \ref{fig:optimal_time_all_cams}, points in the front camera can only be projected to itself and are unable to leverage multi-camera depth estimation. However, we find that multi-timestep aggregation can bring \% of change in object center projection $>$ 1px from 17\% and 0.4\% to 53\% and 22\% for objects at 20m\-40m and 40m\-60m, respectively, significantly decreasing the safety risk of front depth estimation. The numerical values of changes in projected location can be seen in Figure \ref{fig:boxplot_effective_disparities}. As ease of depth estimation isn't simply a binary indicator of "possible" or "not possible", the actual distance between projected locations of two depth hypotheses matters as well. We find that these values increase over various cameras and depths with more temporal aggregation, demonstrating that increased temporal history significantly eases multi-view depth estimation.
